# Supplementary material for: Leveraging Sparse Linear Layers for Debuggable Deep Networks
Source: arXiv:2105.04857 source file (2021-05-11)
Supplement: Supplementary file 1 [file appendix_unknown.tex]

\begin{figure}[t]
    \centering
        \begin{subfigure}{0.48\textwidth}
        \centering
        \includegraphics[width=0.9\columnwidth]{figures/glm/features/bonnet}

        \caption{"Bonnet"}
    \end{subfigure}
    \caption{Visualizations of the most important feature for classifying 
    [TODO 
        class]s in the ImageNet dataset.}

\end{figure}

\begin{figure}[t]
    \centering
    \includegraphics[width=0.8\columnwidth]{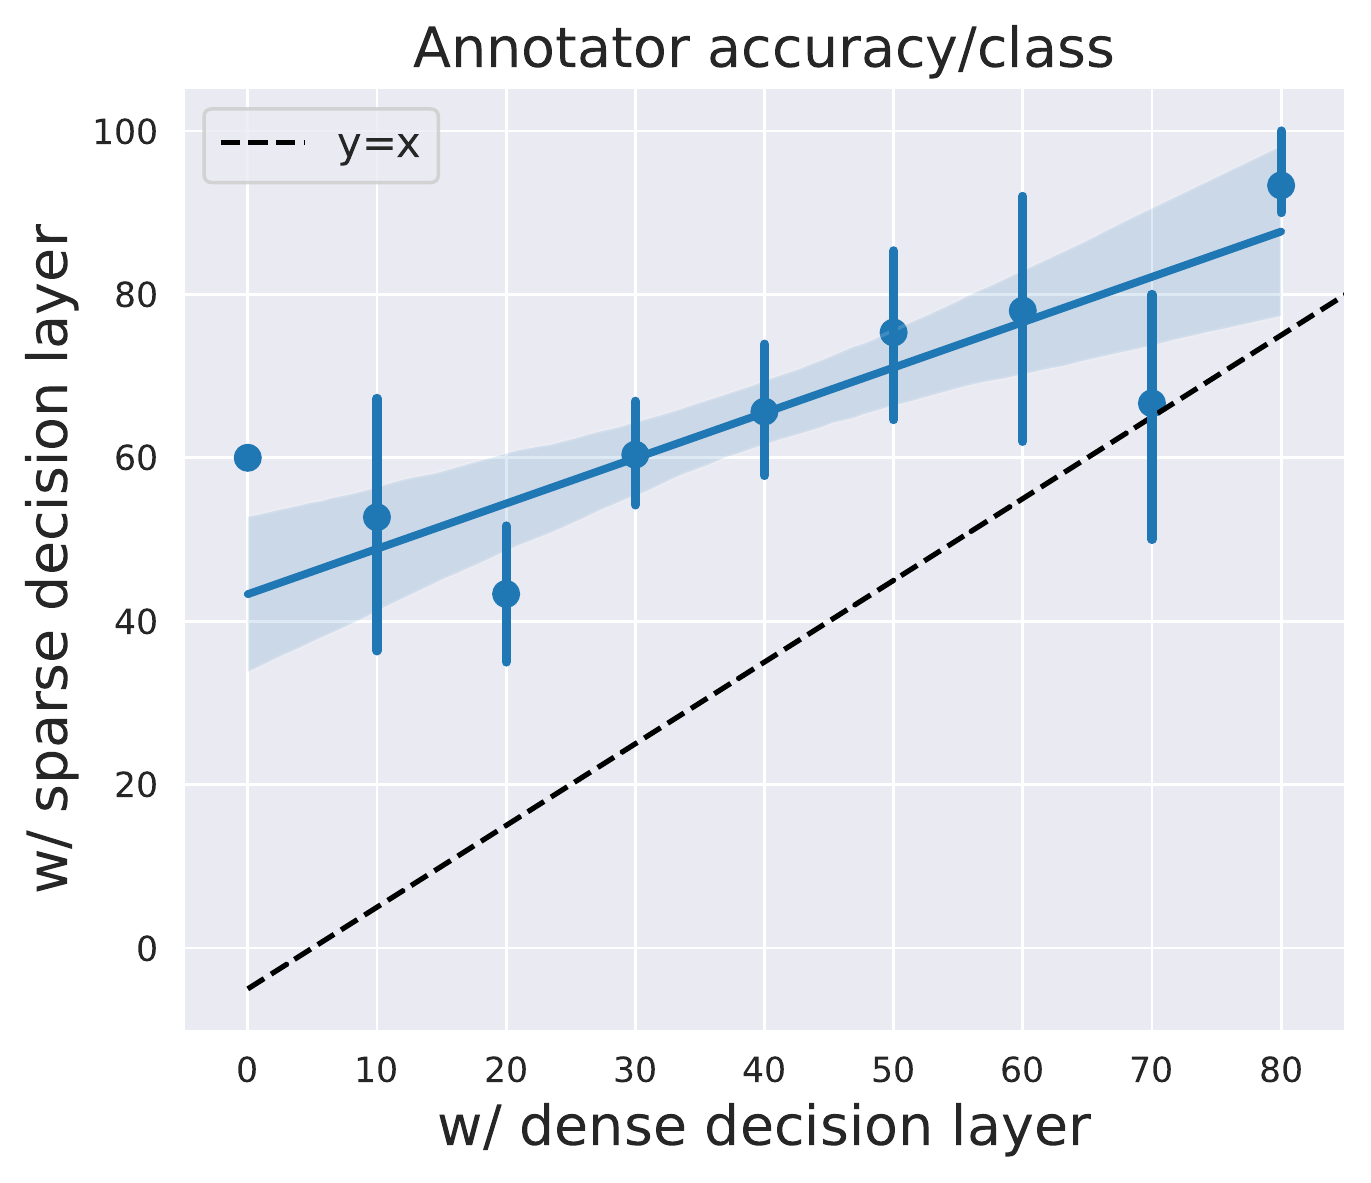}
    \caption{}
    \label{fig:per_class_sim}
\end{figure}
\eric{What is same class vs different class here?}

\begin{figure}[!h]
\centering
\includegraphics[width=1\columnwidth]{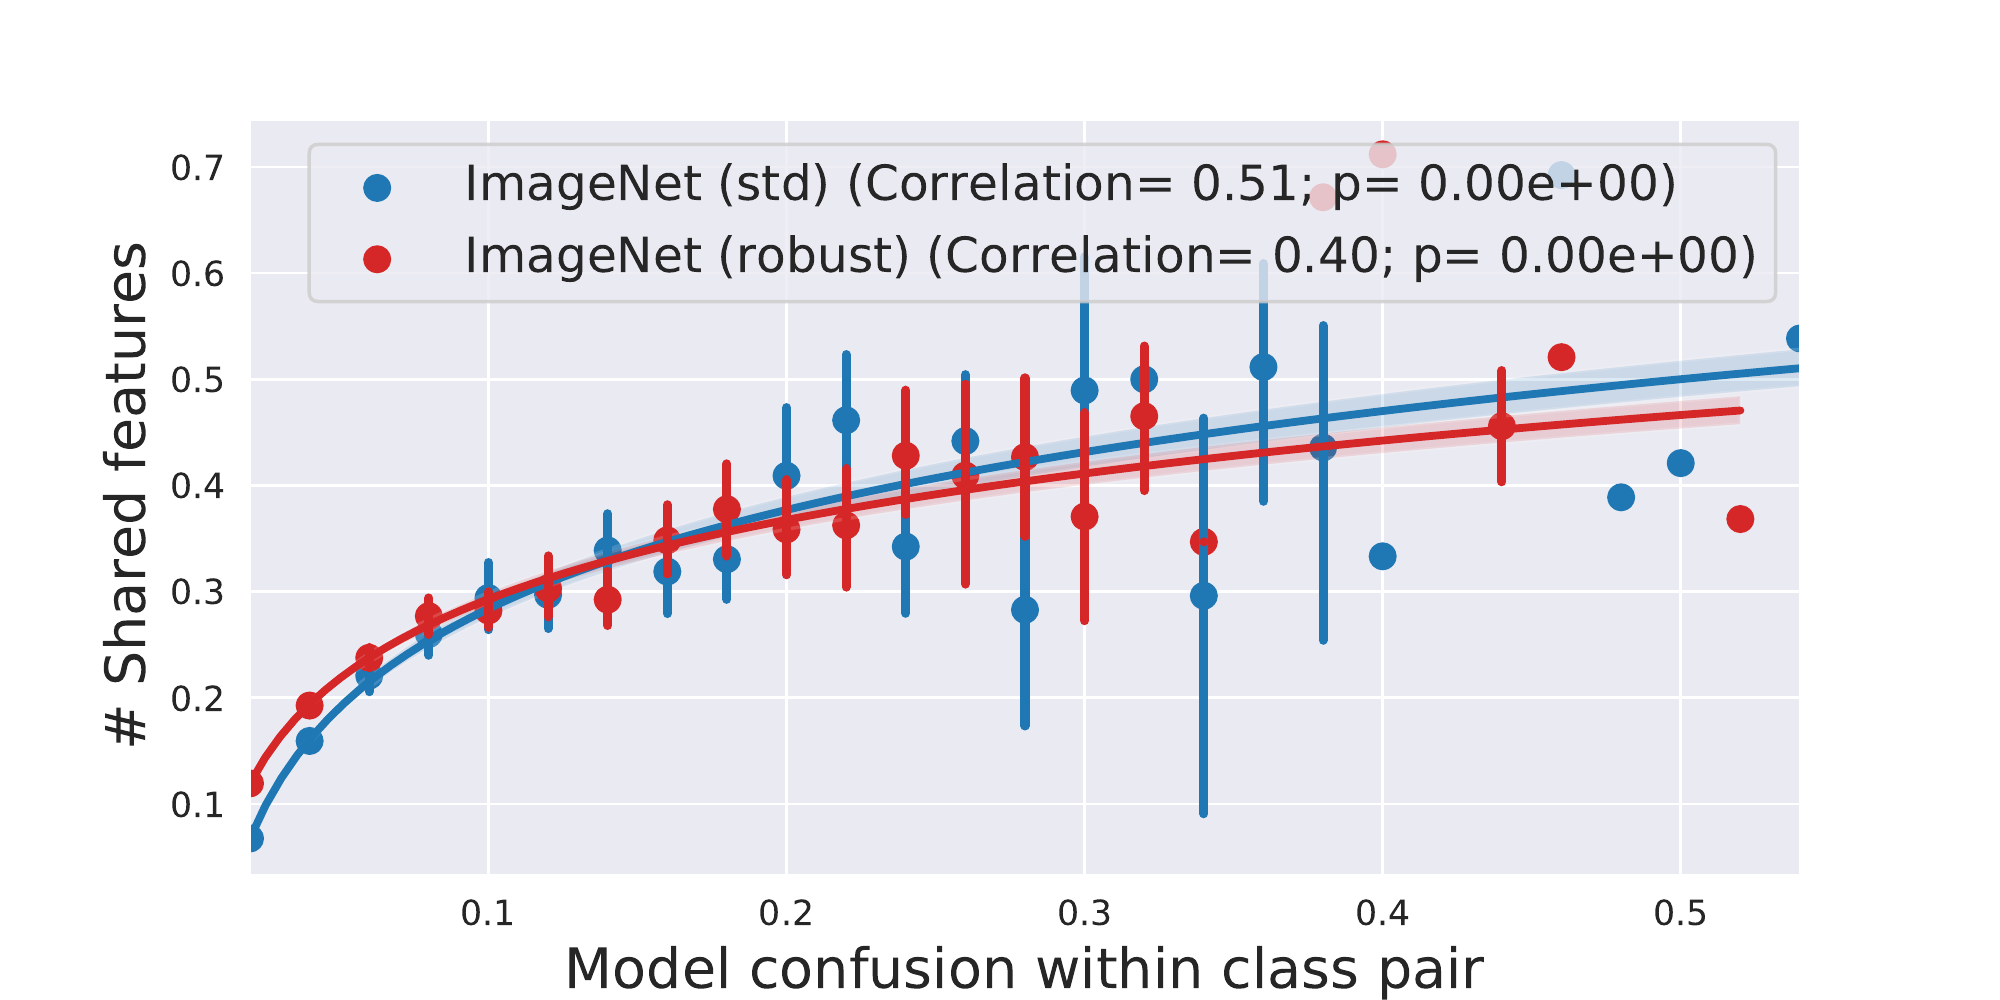}
\caption{}
\label{fig:confusion_correlation}
\end{figure}

\begin{figure}[!h]
    
    \centering
    \includegraphics[width=1\columnwidth]{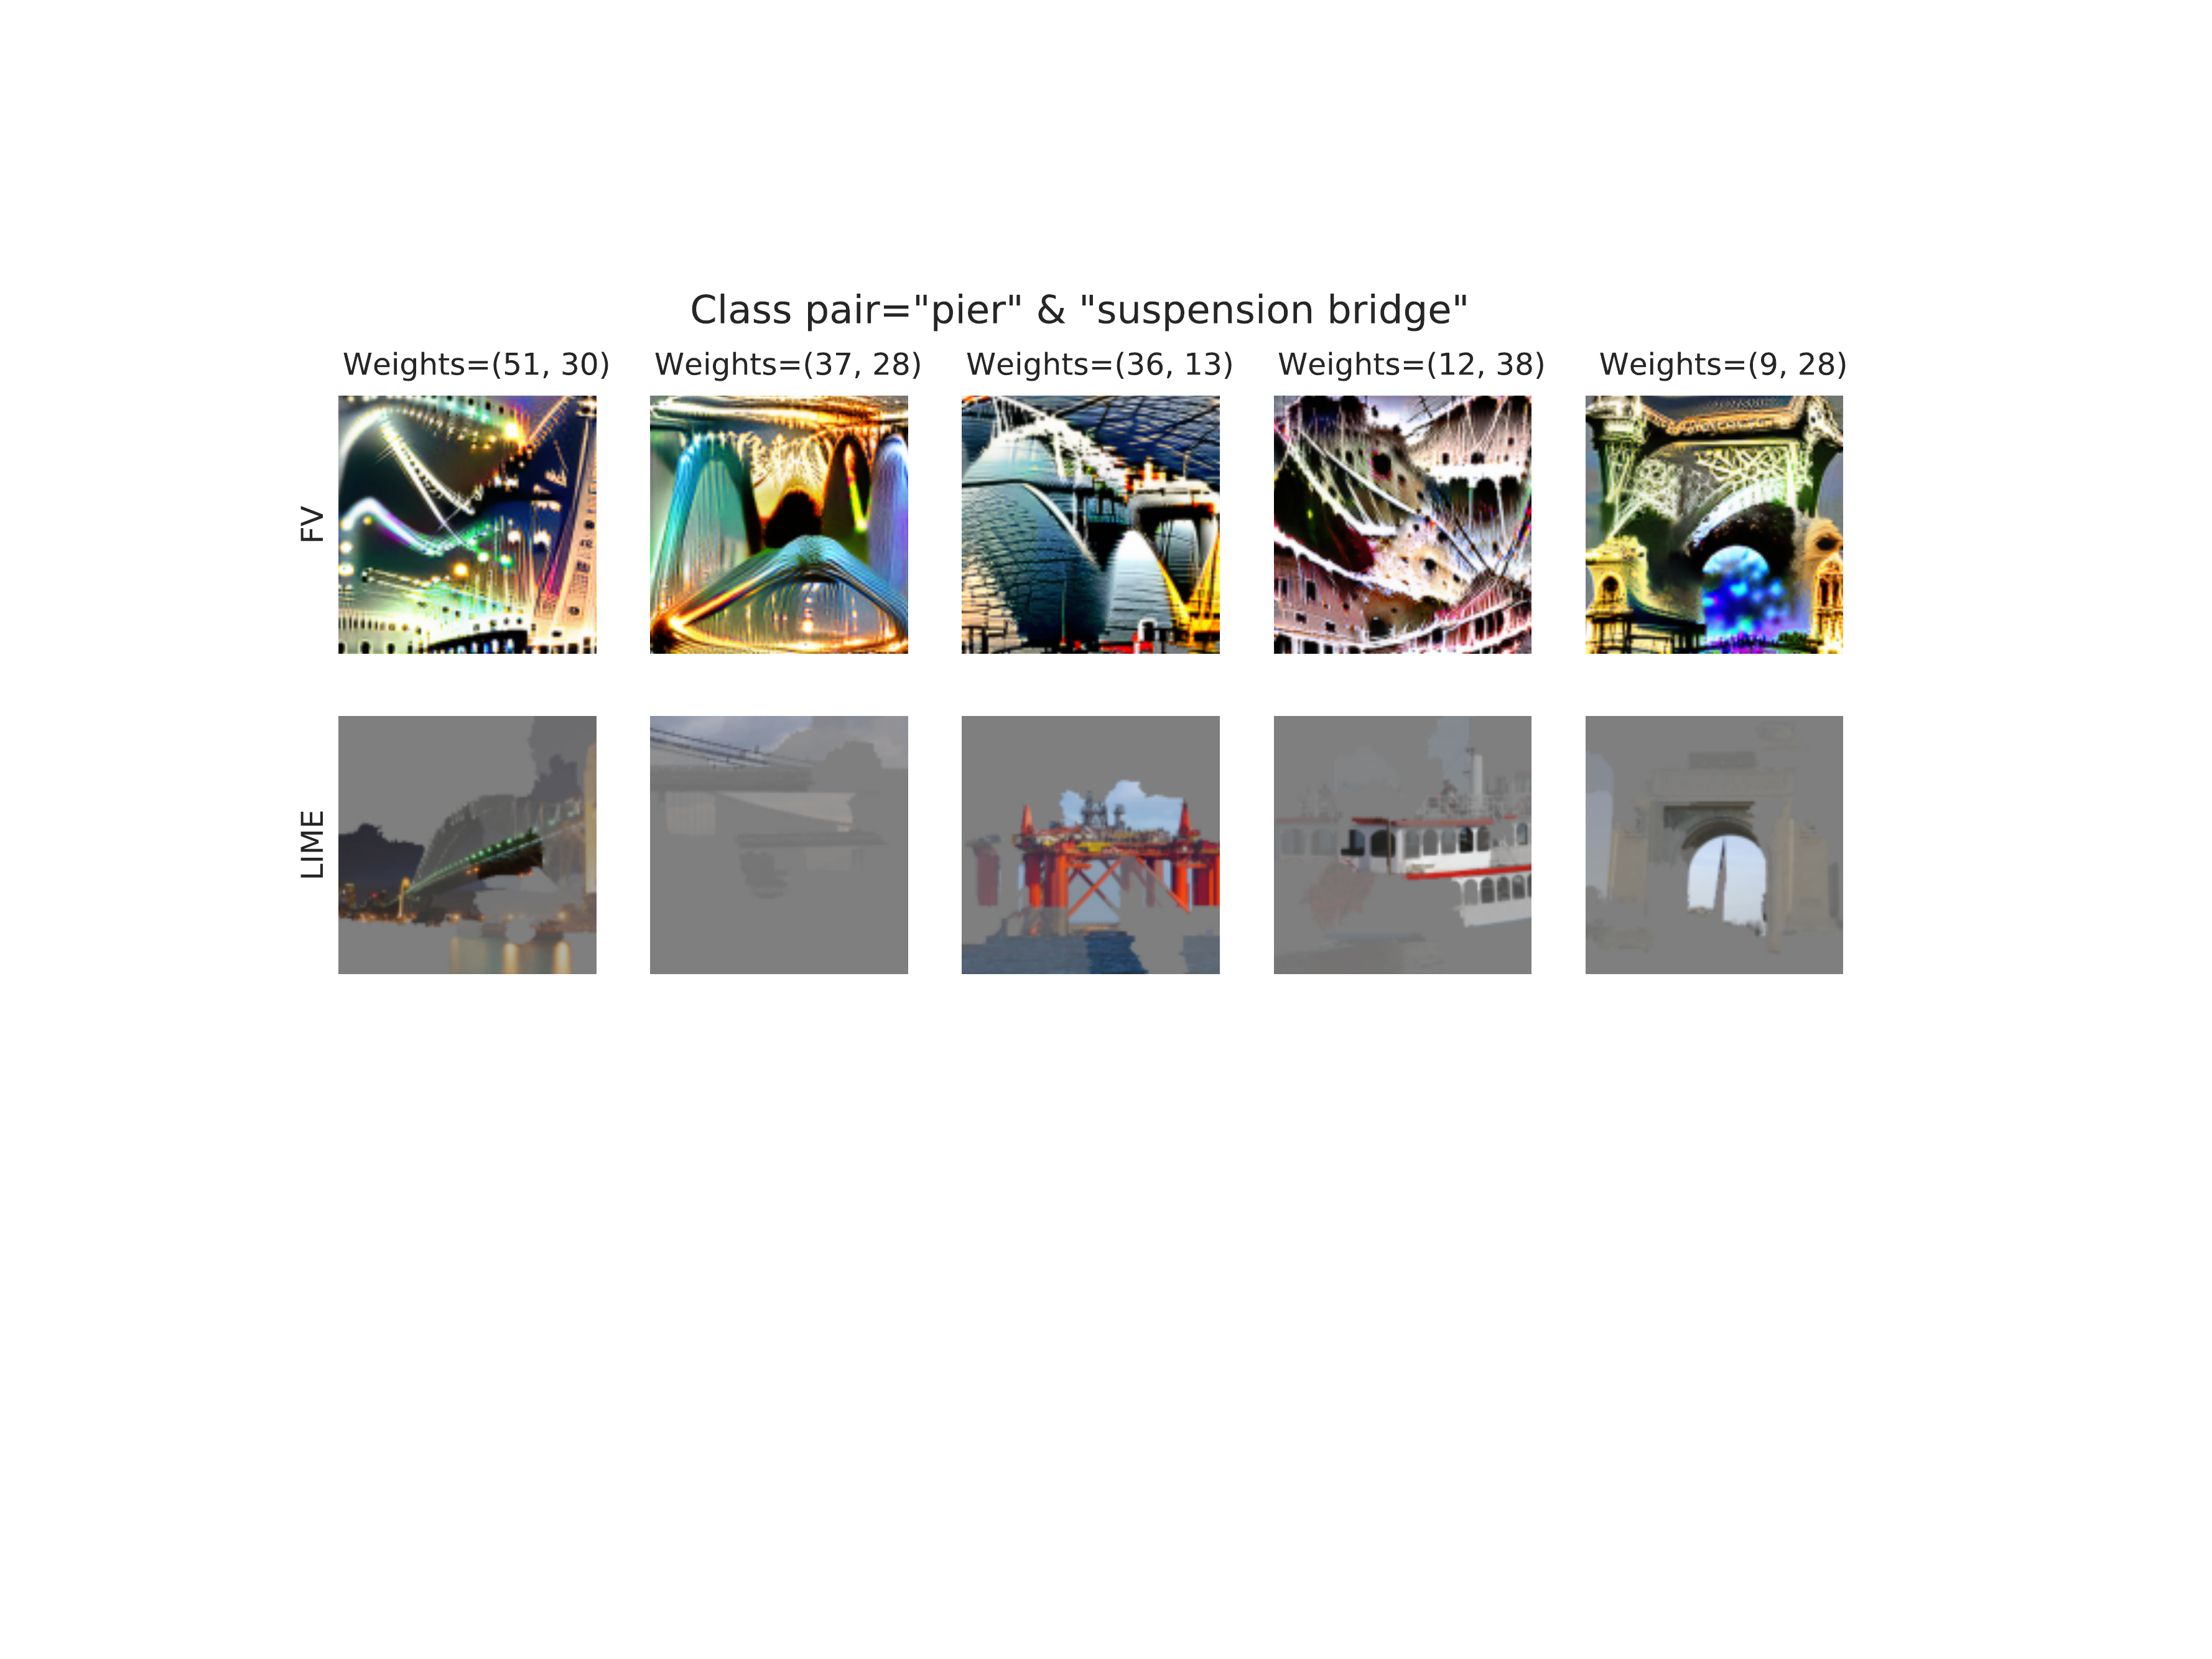}
    \caption{}
    \label{fig:confusion_example}
\end{figure}

\paragraph{Debugging incorrect classifications, and demonstrate how 
    the explanations are different from the local interpretability or example 
    based methods.}
