# Supplementary material for: Leveraging Sparse Linear Layers for Debuggable Deep Networks
Source: arXiv:2105.04857 source file (2021-05-11)
Supplement: Supplementary file 2 [file appendix_vision.tex]

\section{Vision case studies}
\label{app:vision}

\subsection{Spurious correlations}
\label{app:spurious}
